# Supplementary material for: Emergent Multifunctionality in Two-Dimensional Janus VSBrI Monolayer: A Study of Multiferroicity, Magnetoelectricity, and Piezoelectricity
Source: arXiv:2409.02407 source file (2024-09-26)
Supplement: Supplementary file 1 [file Supplemental_Material.pdf]

# Emergent Multifunctionality in Two-Dimensional Janus VSBrI Monolayer: A Study of Multiferroicity, Magnetoelectricity, and Piezoelectricity

*Qiuyue Ma, Busheng Wang, Guochun Yang, and Yong Liu**

*State Key Laboratory of Metastable Materials Science and Technology & Key Laboratory for Microstructural Material Physics of Hebei Province, School of Science, Yanshan University, Qinhuangdao, 066004, P.R. China*

+ corresponding author:
Electronic mail: yongliu@ysu.edu.cn

Table SI. Structural parameters of the Janus VSBrI monolayer.

| Lattice constant | Bond lengths | Bond angles |
| --- | --- | --- |
| a = 3.85 Å<br>b = 4.66 Å | 2.79 Å (V-I)<br>2.60 Å (V-Br)<br>2.11 Å (V-$S_1$)<br>2.55 Å (V-$S_2$) | 180 $^o$ (S-V-S)<br>97.3 $^o$ (I-V-$S_1$)<br>82.6 $^o$ (I-V-$S_2$)<br>97.3 $^o$ (Br-V-$S_1$)<br>82.6 $^o$ (Br-V-$S_2$) |

**A comparison of structural parameters with its parent structure $VSI_2$:**

The V ions are located at the center of the $S_2Br_2I_2$ octahedron and shifts towards S ions on the one side, resulting in different bond lengths of V-S1 (2.11 Å) and V-S2 (2.55 Å), which breaking the spatial inversion symmetry along the *b*-axis and leading to a polar structure. For parent structure $VSI_2$ monolayer, the bond lengths of V-S1 and V-S2 are 2.10 Å and 2.49 Å, respectively, which are shorter than those in the Janus VSBrI monolayer. Consequently, the lattice parameter *b* of Janus VSBrI monolayer is larger than that of the $VSI_2$ ($b$ = 4.60 Å). The V-halogen bond lengths depend on the monolayer's other halogen. Comparing the V-I bond lengths in VSBrI, it decreases with the addition of higher electronegative halogen atoms Br as 2.60 Å, which is lower than the V-I bond lengths in $VSI_2$ of 2.80 Å. The I/Br-V-S1 and I/Br-V-S2 bond angles are larger and smaller, respectively, than the I-V-S1 (96.8$^o$) and I-V-S2 (83.2$^o$) bond angles of the $VSI_2$ monolayer, resulting in the lattice

parameter *a* of the Janus VSBrI monolayer being smaller than that of the parent structure $VSI_2$ ($a$ = 3.99 Å)[1].

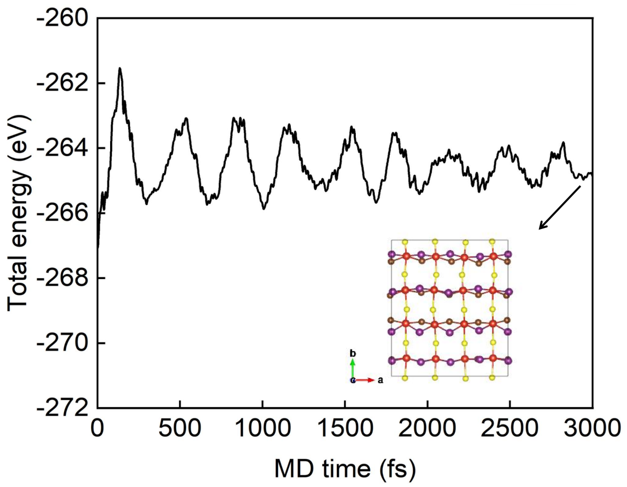


Fig. S1. The fluctuation of total energy during AIMD simulations at 300 K. Inset is the atomic structure of the VSBrI monolayer after a simulation time of 3000 fs.

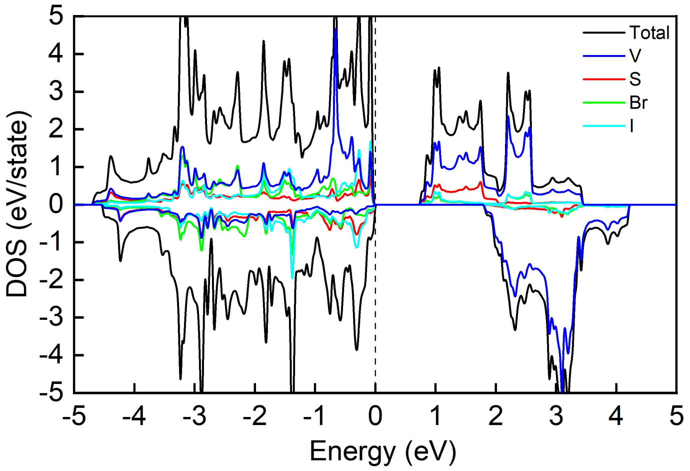


Fig. S2. The projected Density of states (PDOS) of the Janus VSBrI monolayer at the PBE + *U* level.

**Curie temperature simulation:**

Monte Carlo simulations on the basis of 2D Heisenberg Hamiltonian model were carried out, the Hamiltonian is defined as:

$$H = -\sum_{\langle i,j \rangle} J_{ij} S_i S_j - A(S_i^Z)^2 (1)$$

where the $S$ and $A$ represent the spin quantum number ($|S|$=1/2) and the MAE, respectively. The magnetic coupling parameters of the nearest-neighbor $J_1$, next nearest-neighbor $J_2$, and third-nearest-neighbor $J_3$ are calculated via:

$$E(FM) = E_0 - (4J_1 + 4J_2 + 8J_3)S^2 (2)$$

$$E(AFM1) = E_0 - (4J_1 - 4J_2 - 8J_3)S^2 (3)$$

$$E(AFM2) = E_0 - (-4J_1 + 4J_2 - 8J_3)S^2 (4)$$

$$E(AFM3) = E_0 - (-4J_1 - 4J_2 + 8J_3)S^2 (5)$$

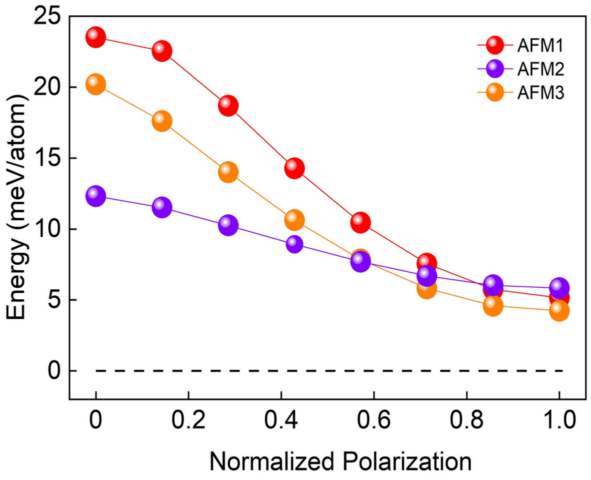


Fig. S3. Relative energy dependence on the polarization in the Janus VSBrI monolayer for four configurations (FM, AFM1, AFM2, AFM3) considered, with the energy of the FM configuration set as the reference zero at a particular polarization. During the calculations, Janus VSBrI monolayer degrees of freedom are fixed at the ground state, except for manually moving the V atom along the V-S chain. A normalized polarization of 1 corresponds to the fully distorted structures (FE phase).

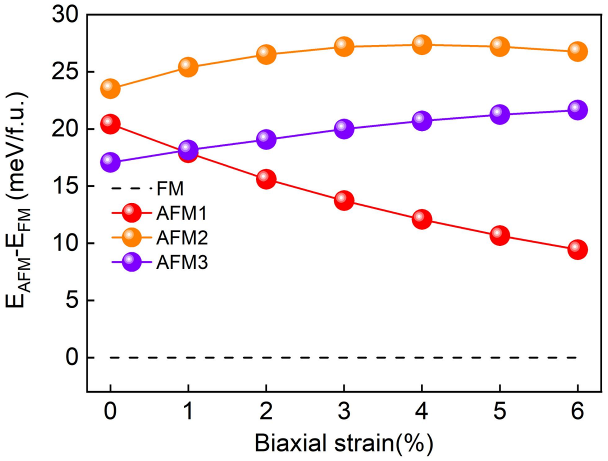


Fig. S4. Energy difference between three AFM and FM configurations of the Janus VSBrI monolayer under biaxial tensile strain ranging from 0% to 6%.

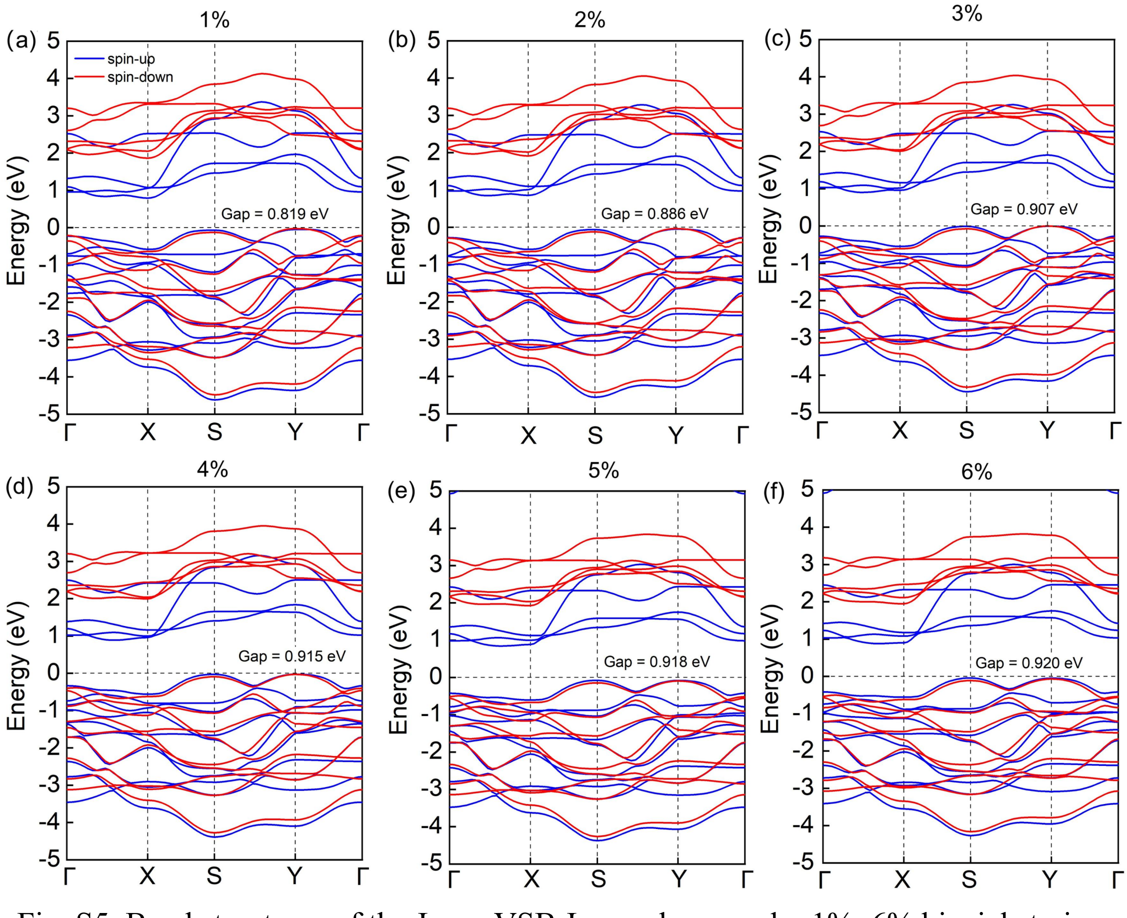


Fig. S5. Band structures of the Janus VSBrI monolayer under 1%~6% biaxial strain.

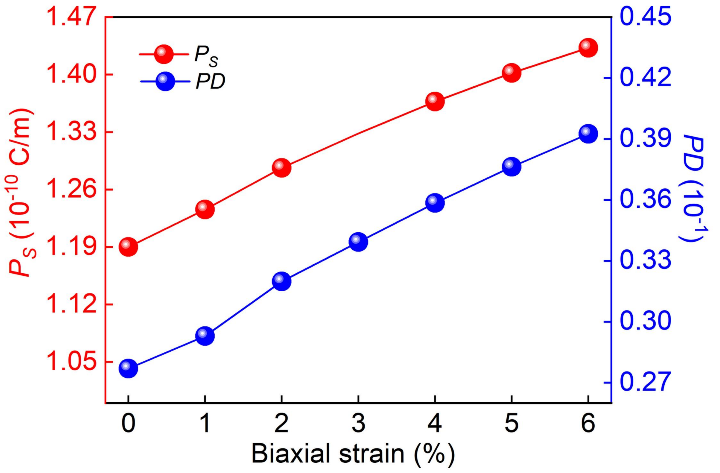


Fig. S6. Spontaneous ferroelectric polarization ($P_S$) and polar displacement ($PD$) of the VSBrI monolayer under biaxial strain ranging from 0% - 6%.

**Piezoelectricity calculations:**

The relaxed piezoelectric tensors ($e_{ij}$ and $d_{ij}$) are obtained as the sum of ionic and electronic contributions:

$$e_{ij} = \frac{\partial P_i}{\partial \varepsilon_j} = e_{ij}^{elc} + e_{ij}^{ion} \quad (6)$$

$$d_{ij} = \frac{\partial P_i}{\partial \sigma_j} = d_{ij}^{elc} + d_{ij}^{ion} \quad (7)$$

where the $P_i$, $\varepsilon_j$, and $\sigma_j$ represent the piezoelectric polarizations, strains, and stresses, respectively. The piezoelectric strain coefficients $d_{ij}$ can be derived by piezoelectric stress coefficients $e_{ij}$ and elastic stiffness coefficients $C_{ij}$:

$$d_{11} = \frac{e_{11}C_{22} - e_{12}C_{12}}{C_{11}C_{22} - C_{12}^2} \quad (8)$$

$$d_{12} = \frac{e_{12}C_{22} - e_{12}C_{12}}{C_{11}C_{22} - C_{12}^2} \quad (9)$$

$$d_{31} = \frac{e_{31}C_{22} - e_{32}C_{12}}{C_{11}C_{22} - C_{12}^2} \quad (10)$$

$$d_{32} = \frac{e_{32}C_{11} - e_{31}C_{12}}{C_{11}C_{22} - C_{12}^2} \quad (11)$$

Table SII. The energy difference of magnetic configurations between FM and three AFM (AFM1, AFM2, and AFM3) in meV per formula unit (f.u.) and the ground magnetic configurations (GMC) for VSBrI under different $U_{eff}$ values (0 ~ 2 eV). Here, $E_{FM}$ is used as the reference for comparing the energies of these configurations.

| | | $E_{AFM1}$-$E_{FM}$ (meV/f.u.) | $E_{AFM2}$-$E_{FM}$ (meV/f.u.) | $E_{AFM3}$-$E_{FM}$ (meV/f.u.) | GMC |
|---|---|---|---|---|---|
| $U_{eff}$ (eV) | 0 | 10.146 | 11.811 | 3.008 | FM |
| | 0.5 | 11.422 | 15.700 | 7.568 | FM |
| | 1 | 13.509 | 18.499 | 10.538 | FM |
| | 1.5 | 17.114 | 21.558 | 14.189 | FM |
| | 2 | 23.176 | 25.668 | 19.247 | FM |

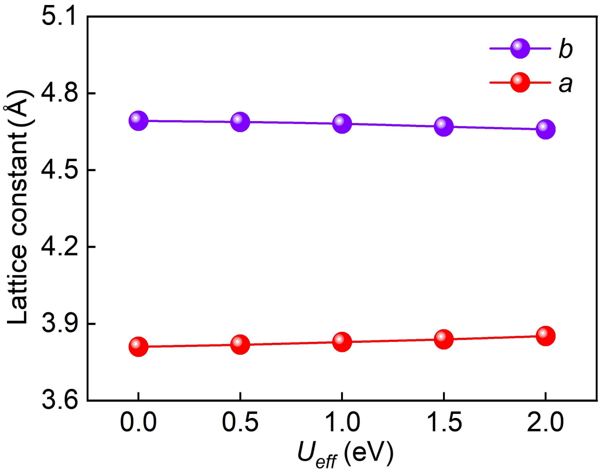


Fig. S7. Spontaneous ferroelectric polarization (*Ps*) and polar displacement (*PD*) as functions of $U_{eff}$ for the Janus VSBrI monolayer.

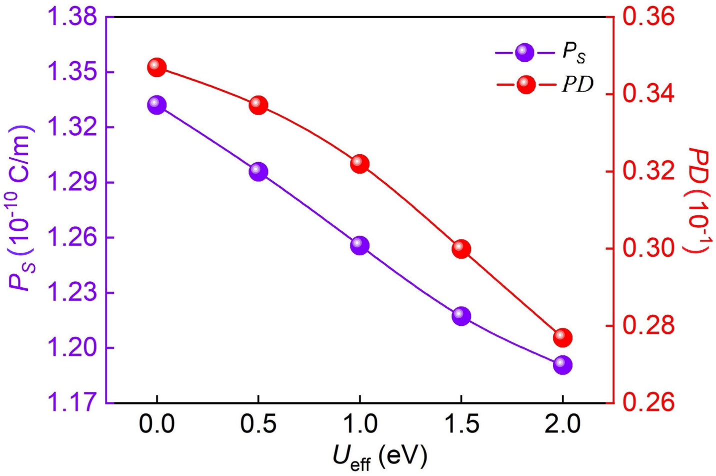


Fig. S8. Lattice constants *a* and *b* as functions of $U_{eff}$ for the Janus VSBrI monolayer.

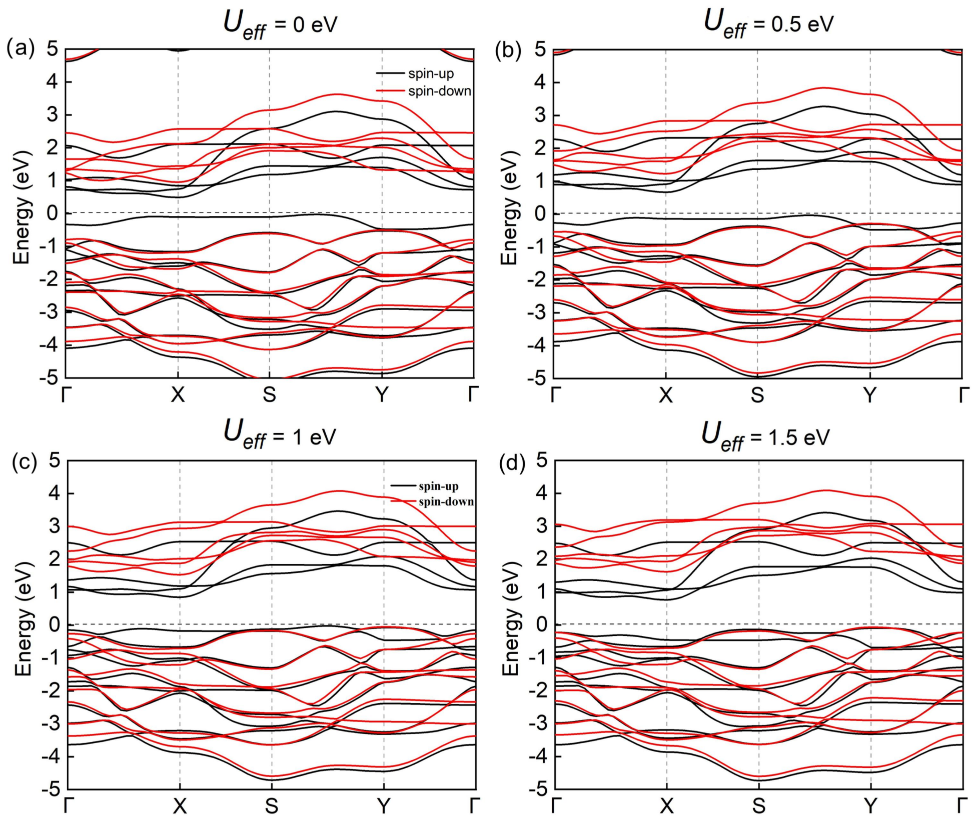


Fig. S9. Band structures of the Janus VSBrI monolayer under different $U_{eff}$ values. (a) 0 eV, (b) 0.5 eV, (c) 1 eV, (d) 1.5 eV.

**The influence of $U_{eff}$ value：**

We listed the energy differences between the FM and three AFM states across the $U_{eff}$ range of 0 to 2 eV in Table SII of the Supplemental Material. The results indicate that the ground state of the Janus VSBrI monolayer is still FM. As shown in Fig. S7, the polar displacement decreases as the $U_{eff}$ increase, indicating that the FE state approaches the PE state, resulting in a reduction in the polarization value. The calculation results indicate that the spontaneous ferroelectric polarization decreases from 1.33 × $10^{-10}$ C/m to 1.20 × $10^{-10}$ C/m. The physical reason for the diminishing ferroelectricity is that the increased $U_{eff}$ weakens the *d-p* orbital hybridization between V and S, thereby reduce the driving force of its proper ferroelectricity. As shown in Fig. S8 of the Supplemental Material, the lattice constants *a* and *b* do not change significantly as the $U_{eff}$ value increases. The band structures of Janus VSBrI monolayer under different $U_{eff}$ value show no obvious alterations, and its semiconductor characteristics remain unaltered [Fig. S9].

[1] D. Li, P. Liu, R. He, Y. Bai, C. Liu, B. Wang, and G. Jia, Appl. Phys. Lett. 123, 052902 (2023).
